# Supplementary material for: Full rotational dynamics of plastic microfibers in turbulence
Source: arXiv:2406.12462 ancillary file (2024-08-01)
Supplement: Supplementary file 1 [file suppl.pdf]

# Full rotational dynamics of plastic microfibres in turbulence: Supplementary material

Vlad Giurgiu,[1] Giuseppe Carlo Alp Caridi,[1] Marco De Paoli,[2,1] and Alfredo Soldati[1,3,*]

[1] *Institute of Fluid Mechanics and Heat Transfer, TU Wien, 1060 Wien, Austria*
[2] *Physics of Fluids Group, University of Twente, 7500AE Enschede, The Netherlands*
[3] *Polytechnic Department, University of Udine, 33100 Udine, Italy*

(Dated: July 19, 2024)

## CONTENT OF THIS FILE

I. Additional details on methodology 1

II. Additional details on fiber properties 1

III. Additional details on rotation rates computation 1

IV. Convergence of the statistics collected 2

V. Influence of curvature on rotation rates and orientation 2

VI. Settling behavior 3

References 4

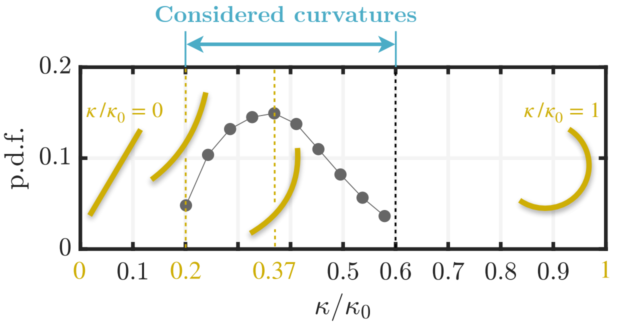


FIG. S1. p.d.f. of dimensionless curvature. Four exemplar fibers (yellow lines) having curvatures of 0, 0.2, 0.37, and 1, are also shown. The range of curvatures considered is indicated by the blue double arrow.

## I. ADDITIONAL DETAILS ON METHODOLOGY

The working fluid is water at the temperature of $15.2\,^\circ\mathrm{C}$ with density $\rho = 1\,\mathrm{g\,cm^{-3}}$ and kinematic viscosity $\nu = 1.13\,\mathrm{mm^2\,s^{-1}}$ [1].

Measurements are performed at two wall-normal locations, $y^+ = y/\delta_\nu < 270$ and $640 < y^+ < 800$ in a volume having dimensions in $x, y$, and $z$ directions of 5.3, 1.6, and 3.1 cm, corresponding to $26.3\,\mathrm{cm^3}$.

The fibers are laser-illuminated and tracked using images from six high-speed cameras acquiring at 800 Hz (additional details on the measurement system are reported in Ref. [2]). On average 137 fibers are found in the measurement volume in each snapshot. In total $2.2 \times 10^4$ trajectories were used, which correspond to $9 \times 10^5$ datapoints. Additional details on the adequacy of the produced database are provided in Sec. IV. The tomographic method described in Ref. [3] was used to reconstruct and track each fiber. Present measurements were improved with respect to Refs. [3, 4] through the addition of two extra viewing directions (i.e., increasing the accuracy on the reconstruction [2, 5]) and by increasing the spatial resolution to 49 vox/mm (i.e., reducing the uncertainty on the orientation). This resolution exceeds the ones used in measurements by Ref. [6] (27 px/mm), [7] (30 px/mm), and [8, 9] (10 px/mm). Additionally, the spatial resolution of the present study corresponding to 2.7 vox/$\delta_\nu$ exceeds the one employed in the particle-resolved simulation performed by Ref. [10] (2.4 cells/$\delta_\nu$).

* alfredo.soldati@tuwien.ac.at

## II. ADDITIONAL DETAILS ON FIBER PROPERTIES

The fibers employed are obtained from Nylon threads, and they fall within a wide range of shapes [3, 4]. We characterize the shape of the fibers employed in the experiments by their normalized curvature, $\kappa/\kappa_0$. In Fig. S1 we provide the probability density function (p.d.f.) of fibers curvature $\kappa$ scaled by $\kappa_0 = \pi/l = 2.62\,\mathrm{mm^{-1}}$, with $\kappa_0$ the equivalent curvature of a semi-circle having circumference equal to the nominal fiber length (for straight fibers $\kappa/\kappa_0 = 0$, for half-circle fibers $\kappa/\kappa_0 = 1$). The most probable dimensionless curvature is 0.37, which corresponds to the fiber shown in Fig. 1 of the main text. In this work, we consider only mildly curved fibers, and therefore we remove from the dataset all fibers with $\kappa/\kappa_0 < 0.2$ and $> 0.6$. By neglecting the straighter fibers we ensure an accurate reconstruction of their shape, and consequently a greater accuracy on the measurement of the spinning rate.

## III. ADDITIONAL DETAILS ON ROTATION RATES COMPUTATION

To compute all fiber rotation rate components we proceed as follows. The components of $\mathbf{e_1}$, $\mathbf{e_2}$, and $\mathbf{e_3}$ in the

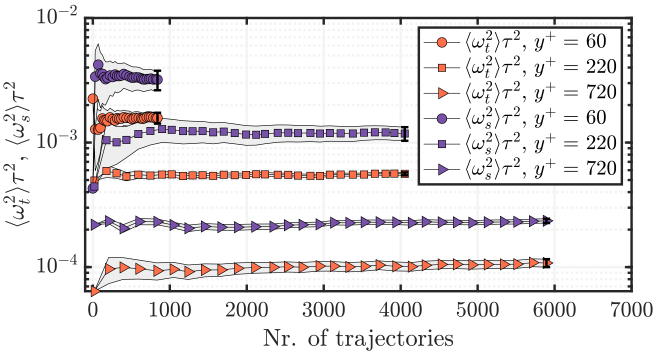


FIG. S2. Convergence of mean squared tumbling (orange) and spinning (violet) rates in three wall-normal bins centered at $y^+ = 60,\ 220,\ 720$ as a function of the number of trajectories considered. Bins are logarithmically spaced over $y^+$. Thickness of the shaded area and error-bar indicate twice the standard deviation of all previous values in each curve.

laboratory reference frame are first filtered using a Robust Locally Weighted Scatterplot Smoothing ('rlowess') [11] filter used also by Refs. [7, 12] to reduce the noise and remove outliers. Following Ref. [6] we choose $15\tau$ as the filter kernel width. Then we build the rotation matrix $\boldsymbol{R} = (\mathbf{e_1}\ \mathbf{e_2}\ \mathbf{e_3})$. Its time derivative $\dot{\boldsymbol{R}}$ is computed with first-order finite differences, with a time-step equal to $0.33\tau_\eta(y^+ = 720)$. The angular velocity matrix in the fiber-fixed reference frame $(\mathbf{e_1},\ \mathbf{e_2},\ \mathbf{e_3})$ is anti-symmetric and obtained as $\boldsymbol{\Omega} = \boldsymbol{R}^{-1}\dot{\boldsymbol{R}}$ [13]. Therefore, the spinning rate is $\omega_s = \Omega_{32}$ and the tumbling rates are $\omega_2 = \Omega_{13}$, $\omega_3 = \Omega_{21}$, and $\omega_t = (\omega_2^2 + \omega_3^2)^{1/2}$ [13]. In the laboratory reference frame, the angular velocity matrix is $\boldsymbol{\Omega}' = \dot{\boldsymbol{R}}\boldsymbol{R}^{-1}$ [13]. Therefore, rotation rates in this frame are $\omega_x = \Omega'_{32}$, $\omega_y = \Omega'_{13}$, and $\omega_z = \Omega'_{21}$.

## IV. CONVERGENCE OF THE STATISTICS COLLECTED

We carried out a convergence study to assess the suitability of our sample size to compute the statistics discussed in the main text, i.e. mean square tumbling and spinning rates over the wall-normal direction. We analyze in Fig. S2 the effect of the number of trajectories considered on the rotation rates measured. Results are shown with respect to three wall-normal and logarithmically spaced bins, centered at $y^+ = 60,\ 220$, and 720. The standard deviation of all values within each curve consistently remained below 18% of the final value.

We assessed the adequacy of our sample size for computing the p.d.f. of the normalized squared tumbling rate, with the results presented in Fig. S3. This analysis demonstrates that randomly selecting only 50% or 10% of the samples has a minimal impact on the overall p.d.f. of the tumbling rate. However, using the complete dataset reveals the strongest tumbling rate events at $\approx 56\langle\omega_t^2\rangle$. When the sample size is reduced by 50% and 90%, the peak events are slightly lower, occurring at $\approx 53\langle\omega_t^2\rangle$ and $51\langle\omega_t^2\rangle$, respectively.

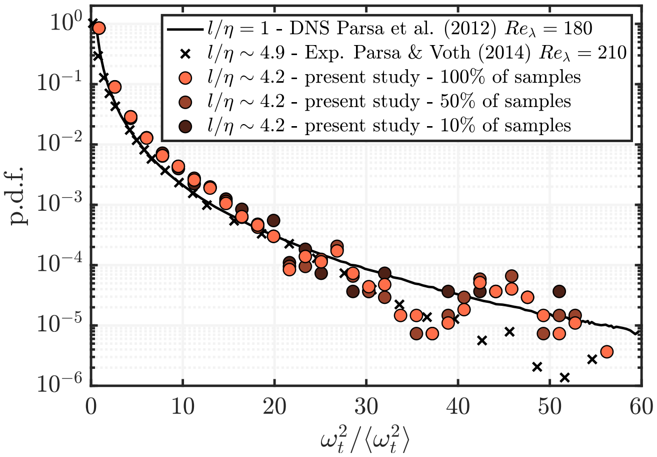


FIG. S3. P.d.f. of the normalized tumbling rate measured in the center of the channel for different number of samples: the full dataset (●), 50% (●), and 10% (●) of the samples compared to numerical simulations of straight rods with $l/\eta = 1$ ([14], black line) and experiments $l/\eta \sim 4.9$ ([15], ×) in HIT. $Re_\lambda$ is the Taylor Reynolds number.

## V. INFLUENCE OF CURVATURE ON ROTATION RATES AND ORIENTATION

All reported results of the main text have been computed using fibers with a dimensionless curvature in the range $0.2 < \kappa/\kappa_0 < 0.6$. These limits have been chosen to restrict the influence of curvature on the results. Nonetheless, the effect of curvature on mean squared tumbling and spinning rates is shown in Fig. S4 for both channel regions. At the channel center, spinning rates show a minimal, non-monotonic behavior with curvature, with the highest curvature bin exhibiting the highest rates. In contrast, tumbling rates slightly decrease in this region with increasing curvature. Near the wall, spinning rates show a slight increase, while tumbling rates reduce minimally with increasing curvature. In the insets of each panel, the deviation of the rotation rates from those of the fibers in the lowest curvature bin is provided. The deviations were observed to be below 25% for both spinning and tumbling, in both channel regions, and for both intermediate and high curvature bins.

We asses the effect of curvature on the p.d.f. of the fiber orientation in both channel regions in Fig. S5. To this aim, we consider the stream-wise component of the unit vector aligned with the longitudinal axis ($e_{1x}$), and the components in the wall-normal ($|e_{2y}|$) and span-wise directions ($|e_{2z}|$) of the unit vector aligned with the transverse axis ($\mathbf{e_2}$). Overall, a negligible effect of curvature on the orientation of the fibers' longitudinal axis and containing plane was found both near the wall ($y^+ < 100$)

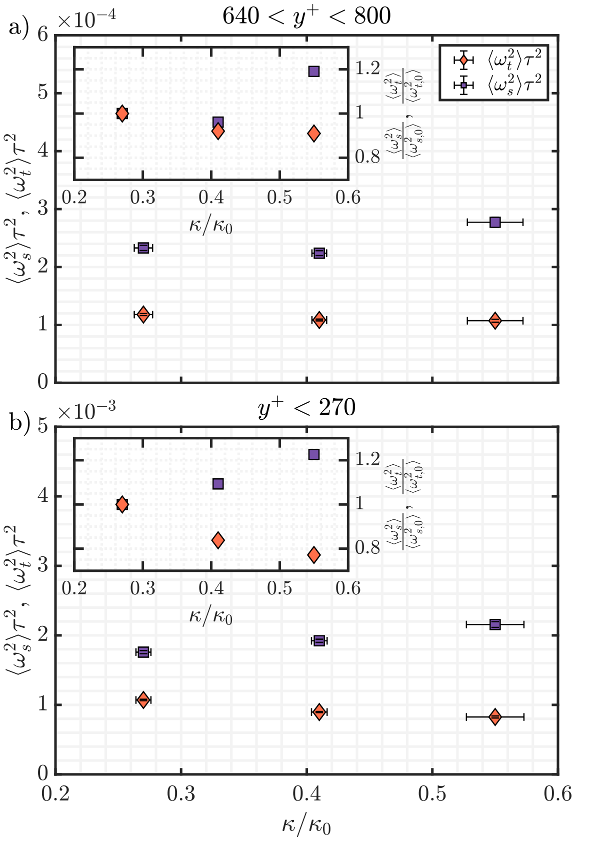


FIG. S4. Mean square tumbling (♦) and spinning (■) rates over dimensionless curvature. Panel a) and b) show data from the channel center ($640 < y^+ < 800$) and near-wall region ($y^+ < 270$), respectively. Here $\langle\cdot\rangle$ represents the average within each bin of $\kappa/\kappa_0$. The bin width is $0.14\kappa/\kappa_0$. The abscissa of panel b) is also valid for a). The legend of panel a) is also valid for b). The horizontal and vertical error-bars correspond to confidence intervals at 99% confidence level. The insets show the mean square tumbling and spinning rates scaled by those of the lowest curvature bin, $\langle\omega_{t,0}^2\rangle$ and $\langle\omega_{s,0}^2\rangle$, respectively.

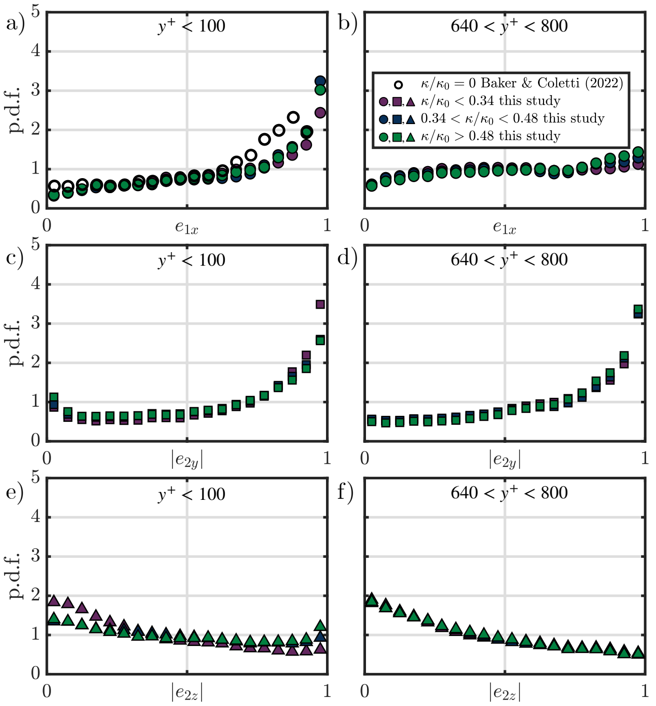


FIG. S5. The p.d.f. of $e_{1x}$, $|e_{2y}|$, and $|e_{2z}|$ for different fiber curvature classes are shown in panels a) and b), c) and d), and e) and f), respectively. The curvature classes are the same as in Fig. S4. Panels a), c), and e) show data near the wall ($y^+ < 100$) and b), d), and f) from the central channel region ($640 < y^+ < 800$). The legend of b) is valid for all panels. Present data is compared to straight rods in a turbulent boundary layer ([6], **O**) in panel a). All bins have a width of 0.05. The ordinate axes of panels a), c), and e) are also valid for panels b), d), and f).

and at the channel center. Nonetheless, a slight dependence on curvature was found near the wall for the $|e_{2z}|$ component, with fibers in the lowest curvature bin showing a reduced alignment of $\mathbf{e_2}$ with the span-wise direction.

## VI. SETTLING BEHAVIOR

The fibers are negatively buoyant in water at a temperature of 15.2 °C with a mass density ratio $\mathcal{R} = \rho_f/\rho = 1.15$. To determine whether their settling behavior affects the statistics on rotation rates and orientation presented in Fig. 2, 3, 4, and 5*c* and Fig. 5*a* and *b*, respectively, we follow the reasoning of Ref. [16]. The half-length of the fibers is $a_\parallel = l/2 = 0.6 \times 10^{-3}$m and the half-diameter is $a_\perp = d/2 = 5 \times 10^{-6}$m. The aspect ratio is $\lambda = a_\parallel/a_\perp = 120$ and the fiber's volume is $V_p = (4\pi/3)a_\perp^2 a_\parallel = 6.28 \times 10^{-14}\mathrm{m}^3$. The non-dimensional volume is $\mathcal{V} = gV_p/\nu^2 = 0.48$, where $g = 9.81\,\mathrm{m/s}^2$ is the gravitational acceleration. The linear particle size is $a = \max\{a_\parallel, a_\perp\}$. In the limit of small settling velocities, the particle Reynolds number is $Re_p = av_g/\nu \sim \mathcal{R}\mathcal{V}/(6\pi) = 0.03$ [16], where $v_g$ is the settling velocity, which amounts to $v_g = Re_p\nu/a \sim 5.5\times10^{-5}\mathrm{m\,s}^{-1}$. The ratio of the shear velocity to this estimated settling velocity is $u_\tau/v_g \sim 370$, implying a negligible settling velocity with respect to the expected fiber velocities in the present flow conditions. Following Ref. [16], the particle relaxation time is $\tau_p = (2\rho_f/(9\rho))\,a_\perp a_\parallel/\nu = 0.68\,\mathrm{ms}$. The Stokes number with respect to the smallest Kolmogorov time-scale (at $y^+ = 0$, $\tau_{0,\eta} = 5.7\,\mathrm{ms}$) is $St_{0,\eta} = \tau_p/\tau_{0,\eta} = 0.12$, implying a translational tracing behavior. The non-dimensional settling velocity is $V_g = v_g/(g\tau_p) = 8.3 \times 10^{-3}$. The orientation of settling, non-spherical particles does not oscillate if $1 - \mathit{\Delta} < 1$ [16], with $\mathit{\Delta} = 1 - 4(V_g^*)^2 C_T|h(\lambda)|\mathcal{R}^3\mathcal{V}^2$. For large $\lambda$, $|h(\lambda)|\mathcal{R}^3\mathcal{V}^2$ scales with $a_\perp^6$ [16] and we assume a torque coefficient $C_T = 0.5$, if we consider $\lambda = 5$ for particles

in group I from Ref. [16]. Finally, we find $1 - \mathit{\Delta} \sim 0$, implying a non-oscillatory settling behavior of the fibers in quiescent conditions [16].

---


[1] M. Kind and H. Martin, VDI-Wärmeatlas (2013).

[2] V. Giurgiu, G. C. A. Caridi, M. Alipour, M. De Paoli, and A. Soldati, The TU Wien Turbulent Water Channel: Flow control loop and three-dimensional reconstruction of anisotropic particle dynamics, Rev. Sci. Instrum. **94** (2023).

[3] M. Alipour, M. De Paoli, S. Ghaemi, and A. Soldati, Long non-axisymmetric fibres in turbulent channel flow, J. Fluid Mech. **916**, A3 (2021).

[4] M. Alipour, M. De Paoli, and A. Soldati, Influence of Reynolds number on the dynamics of rigid, slender and non-axisymmetric fibres in channel flow turbulence, J. Fluid Mech. **934**, A18 (2022).

[5] G. E. Elsinga, F. Scarano, B. Wieneke, and B. W. van Oudheusden, Tomographic particle image velocimetry, Exp. Fluids **41**, 933 (2006).

[6] L. J. Baker and F. Coletti, Experimental investigation of inertial fibres and disks in a turbulent boundary layer, J. Fluid Mech. **943**, A27 (2022).

[7] S. Shaik, S. Kuperman, V. Rinsky, and R. van Hout, Measurements of length effects on the dynamics of rigid fibers in a turbulent channel flow, Phys. Rev. Fluids **5**, 114309 (2020).

[8] L. Jiang, Private Communication on the "Rotation of anisotropic particles in Rayleigh–Bénard turbulence" published in J. Fluid Mech., Volume 901, Page A8, 2020. (2024).

[9] L. Jiang, E. Calzavarini, and C. Sun, Rotation of anisotropic particles in Rayleigh–Bénard turbulence, J. Fluid Mech. **901**, A8 (2020).

[10] M. Do-Quang, G. Amberg, G. Brethouwer, and A. V. Johansson, Simulation of finite-size fibers in turbulent channel flows, Phys. Rev. E **89**, 013006 (2014).

[11] W. S. Cleveland, Robust locally weighted regression and smoothing scatterplots, J. Am. Stat. Assoc. **74**, 829 (1979).

[12] S. Shaik and R. van Hout, Kinematics of rigid fibers in a turbulent channel flow, Int. J. Multiphas. Flow **158**, 104262 (2023).

[13] K. M. Lynch and F. C. Park, *Modern robotics* (Cambridge University Press, 2017) p. 77.

[14] S. Parsa, E. Calzavarini, F. Toschi, and G. A. Voth, Rotation rate of rods in turbulent fluid flow, Phys. Rev. Lett. **109**, 134501 (2012).

[15] S. Parsa and G. A. Voth, Inertial range scaling in rotations of long rods in turbulence, Phys. Rev. Lett. **112**, 024501 (2014).

[16] T. Bhowmick, J. Seesing, K. Gustavsson, J. Guettler, Y. Wang, A. Pumir, B. Mehlig, and G. Bagheri, Inertia induces strong orientation fluctuations of nonspherical atmospheric particles, Phys. Rev. Lett. **132**, 034101 (2024).
